# Supplementary material for: Class Is Invariant to Context and Vice Versa: On Learning Invariance for Out-Of-Distribution Generalization
Source: arXiv:2208.03462 source file (2025-10-12)
Supplement: Supplementary file 1 [file appendix.pdf]

# Supplementary Materials for “Class Is Invariant to Context and Vice Versa: On Learning Invariance for Out-Of-Distribution Generalization”

This supplementary material will provide further details for the main paper, including A. Theoretical justifications, B. More experimental details, C. More quantitative results, D. More qualitative results. Specifically, **A.1** is for the preliminary knowledge about group theory and causal graph, which we will use to justify the disentanglement of class and context and to define the classification; **A.2** is for proving the disentanglement between  $\mathbf{x}_c$  and  $\mathbf{x}_t$ ; **A.3** is for justifying that Inverse Probability Weighting can realize robust classification; **A.4** is for justifying that IRMCon can achieve  $\phi_t(x) = x_t$ ; **B.1** is for more dataset details; **B.2** is for more implementation details; **B.3** provides more analysis for the Fig. 6. and Fig. 7. in the main paper and how does our IRMCon-IPW superior to traditional context estimation methods; **C.1.** is for illustrating the reproduced results on context biased datasets; **C.2** is for illustrating the bad performance of vanilla ERM (without strong augmentations); **C.3** is for illustrating the domain gap results with pretrained backbone (for complement); **D** is for illustrating the successful cases of our IRMCon and IRMCon-IPW; We summarize our algorithm at the end of Section A.

## A Theoretical Justifications

### A.1 Preliminaries

**Notations.** In group theory, we use capital letters to denote sets and lowercase letters to denote elements.  $\rightarrow$  is the mapping between sets,  $\mapsto$  the mapping between elements.  $\times$  is the Cartesian Product. In the causal graph, capital letters denote variables and corresponding lowercase letters denote their values.

**Group.** A group is a nonempty set  $G$  equipped with a binary operation  $(g_1, g_2) \mapsto g_1g_2$  (we omit the symbol of the operation), where  $g_1, g_2 \in G$ , satisfying the following four axioms: *Closure*:  $\forall g_1, g_2 \in G, g_1g_2 \in G$ ; *Identity*: There exists an identity element  $e \in G$  such that  $\forall g \in G, eg = ge = g$ ; *Inverse*: If  $g \in G$ , there exists an inverse element  $g^{-1} \in G$  such that  $gg^{-1} = g^{-1}g = e$ ; *Associativity*:  $\forall g_1, g_2, g_3 \in G, (g_1g_2)g_3 = g_1(g_2g_3)$ .

**Subgroup.** A subset of group  $G$ , which forms a group, is a subgroup. Additionally, if  $H$  is the subgroup of  $G$ , and  $ghg^{-1} \in H$  for all  $g \in G, h \in H$ , call  $H$  is a normal subgroup.

**Direct Product.** Given two groups  $G$  and  $H$ , the direct product  $G \times H$  is defined as a new set containing the ordered pairs  $(g, h)$ , where  $g \in G, h \in H$  equipped with component-wise binary operation:  $(g_1, h_1) \cdot (g_2, h_2) = (g_1g_2, h_1h_2)$ . This new set satisfies group axioms.

**Quotient Group.** If  $W = G \times H$ ,  $G$  is equivalent to the normal subgroup of  $W$  and  $H$  is equivalent to its corresponding quotient group, i.e.,  $H = W/G$ , where “=” is group isomorphism (the equivalent relation between groups in group theory).

**Group Action.**  $G$  is a group and  $D_x$  is a set, then a (left) group action  $\alpha$  of  $G$  on  $D_x$  is a function  $\alpha: G \times D_x \rightarrow D_x$ , which satisfies the following two axioms: *Identity*:  $\alpha(e, x) = x, e \in G, \forall x \in D_x$ ; *Compatibility*:  $\alpha(g, \alpha(h, x)) = \alpha(gh, x), \forall g, h \in G, \forall x \in D_x$ . We will use  $g \cdot x$  as the abbreviation of  $\alpha(g, x)$ .

**Transitive and Equivalence Relation.** Given a group  $G$  and a set  $D_x$ , if  $\forall x_i, x_j \in D_x, \exists g \in G, g \cdot x_i = x_j$ , we call the action is transitive,  $x_i$  and  $x_j$  have equivalence relation.

**Orbit.** Considering a group  $G$  acting on a set  $D_x$ , the orbit of an element  $x \in D_x$  is defined as:  $G \cdot x = \{g \cdot x \mid g \in G\}$ .

**Group Representation.** A group representation of a group  $G$  on a vector space  $V$  over a field  $F$  is a mapping (group homomorphism),  $\rho: G \rightarrow GL(V)$ , such that  $\rho(g_1 g_2) = \rho(g_1) \rho(g_2)$ , where  $GL(V)$  is the general linear group on  $V$ . Note that the linear group action  $\beta: GL(V) \times V \rightarrow V$  preserves the linear structure:

$$\begin{aligned} \rho(g)(kv_1 + v_2) &= k\rho(g)(v_1) + \rho(g)(v_2), \\ v_1, v_2 \in V, g \in G, k \in F, \end{aligned} \tag{1}$$

where we omit the group action notation  $\cdot$  for brevity.

**Stabilizer.** Given a group element  $g$  and an element  $x_i$  from the acted set  $D_x$ , if  $gx_i = x_i$ , we call this  $g$  is a stabilizer for  $x_i$ .

**Kernel.** The kernel of a mapping (group homomorphism), e.g.,  $\rho: G \rightarrow GL(V)$  is the set of all elements of  $G$  which are mapped to the identity element of  $GL(V)$ :

$$\text{Ker}(\rho) = \{g \in G : \rho(g) = e_{GL(V)}\}. \tag{2}$$

**Causal Graph.** Causal graph [10] indicates how the variables interact with each other to reveal the causal relationships between them. In general, it is denoted by a directed acyclic graph  $\mathcal{G} = \{\mathcal{N}, \mathcal{E}\}$ , including nodes and directed links, where nodes  $\mathcal{N}$  denote variables and directed links  $\mathcal{E}$  denote causal relationships between variables. For example, Fig. 1,  $H \rightarrow (X_0, X)$  denotes the value of the pair is caused by the value of  $H$ ,  $X = hX_0$ . For other basic concepts in causal graph like confounder, intervention and backdoor adjustment, please refer to [10].

## A.2 Why are class features and context features disentangled?

**All real-world transformations form a group  $W$ .** In the real world, there are lots of transformations for an object. For example, “become white”, “become sheep” and “turn 90 degrees”. Actually, they form a group  $W$ , using *combination* as its binary operation. This can be verified by the group axioms, like the combination of “become white” and “become sheep” is still a transformation in  $W$  (*Closure* axiom). There exists identity transformation “no change” in  $W$  (*Identity* axiom). The left 2 axioms can be verified in the same way.

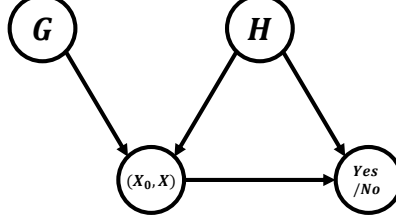

**Fig.1.** Causal Graph for classification, derived from orbit theory.  $H$  and  $G$  are class-agnostic and class-related transformation variables, respectively.  $(X_0, X)$  denotes paired image variable, where  $X = ghX_0$ . “Yes/No” denotes whether  $X$  and  $X_0$  have equivalent relation.

**Decompose  $W$  to  $G$  and  $H$ .**  $W$  can be divided into class-related transformations and class-agnostic transformations according to whether the class of object changes when applying the transformation. We use  $G$  and  $H$  to denote the class-related set and class-agnostic set respectively, and they are also groups. For example, any combination of two class-agnostic transformations from  $H$  is still in  $H$  (*Closure* axiom), and other axioms can be verified. Therefore,  $G, H$  are subgroups of  $W$ . As all transformations can be denoted as class-related, class-agnostic or the combination of them,  $G \times H$  can denote any transformation, *i.e.*, equal to  $W$ . Therefore, if we treat  $G$  as the subgroup,  $H$  is the corresponding quotient group  $H = W/G$ .

The transformation in  $G$  is **disentangled** with the transformation in  $H$ , because the change of each one will not influence another one, according to their definitions (The class-related transformations will not influence the class-agnostic transformations). From the property of  $G$  and  $H$ , we have:

**Theorem 1.** *The disentanglement between  $\mathbf{x}_c$  (class-related feature) and  $\mathbf{x}_t$  (class-agnostic/context feature) is from the disentanglement of their corresponding groups, *i.e.*,  $G$  (class-related transformation group) and  $H$  (class-agnostic transformation group).*

**Proof.** As  $\mathbf{x}_c$  and  $\mathbf{x}_t$  are in vector space,  $G$  and  $H$  are semantic transformation groups, which can act on the object in a semantic way. To prove the theorem, we need to use group representation to map  $G$  and  $H$  into vector space and define the group action on the vector space.

First we define the group action  $\alpha$  for  $W$  on the set  $D_x$  in a semantic way:

$$\alpha : W \times D_x \rightarrow D_x. \quad (3)$$

$$\begin{array}{ccc}
W \times D_x & \xrightarrow{\alpha} & D_x \\
e_W \times g^{-1} \downarrow & & \downarrow g^{-1} \\
W \times V & \xrightarrow{\beta} & V
\end{array}$$

**Fig. 2.** The equivariant map between  $\alpha$  and  $\beta$ .

Then, we define two group representations corresponding to  $H$  and  $G$ :

$$\begin{aligned}
\rho_1 : W &\rightarrow GL(V_1), \text{Ker}(\rho_1) = H, \\
\rho_2 : W &\rightarrow GL(V_2), \text{Ker}(\rho_2) = G,
\end{aligned} \tag{4}$$

and two maps:

$$\begin{aligned}
g^{-1} : D_x &\rightarrow V, V = V_1 \oplus V_2. \\
\beta : W \times V &\rightarrow V, \\
\beta(w, g^{-1}(x)) &= \text{Diag}(\rho_1(w), \rho_2(w))g^{-1}(x),
\end{aligned} \tag{5}$$

where  $w \in W, x \in D_x$ ,  $\text{Diag}$  is the diagonal block matrix, we use  $g^{-1}$  to represent the mapping from  $D_x$  to  $V$  is because we define  $x = g(\mathbf{x}_c, \mathbf{x}_t)$  in the main paper. We use  $\rho_1(w)$  to denote the matrix because  $GL(V)$  (general linear group) is isomorphic to  $GL_n(V)$  ( $n$ -dimensional invertible matrix group). It is easy to prove that  $\beta$  is a group action, where the operation is matrix multiplication.

As  $\beta$  is a group action of  $W$  on  $V$ , with the function  $g^{-1} : D_x \rightarrow V$ , there exists a 1-to-1 mapping between  $\alpha : W \times D_x \rightarrow D_x$  and  $\beta : W \times V \rightarrow V$ , which is illustrated in Fig. 2.

Through the map, we know that any group action by  $w \in W$  on an element  $x \in D_x$  has a corresponding representation described by  $\beta$  in (5) with the mapping function  $g^{-1}$ , which is:

$$\begin{aligned}
\beta(w, g^{-1}(x)) &= \begin{pmatrix} \rho_1(w) \\ \rho_2(w) \end{pmatrix} g^{-1}(x) \\
&= \begin{pmatrix} \rho_1(g) \\ \rho_2(h) \end{pmatrix} (g^{-1}(x)_{V_1} \oplus g^{-1}(x)_{V_2}) \\
&= \rho_1(g)g^{-1}(x)_{V_1} \oplus \rho_2(h)g^{-1}(x)_{V_2}, \\
&= \rho_1(g)\mathbf{x}_c \oplus \rho_2(h)\mathbf{x}_t.
\end{aligned} \tag{6}$$

Eq. (6) denotes that subgroup  $G$  and its quotient group  $H$  separately act on their corresponding subspace  $V_1$  and  $V_2$ , influencing  $\mathbf{x}_c$  and  $\mathbf{x}_t$  respectively. That means the changes of  $\mathbf{x}_c$  are only decided by  $G$ , which is disentangled to  $H$ , the  $\mathbf{x}_t$ 's influencer. Therefore,  $\mathbf{x}_c$  and  $\mathbf{x}_t$  are disentangled.

### A.3 Why does IPW realize robust classification?

We first define the classification in a group orbit view. Then, we draw the causal graph for classification according to the equivalence relation.

**Classification by H-Orbit.** According to Eq. (3), for the quotient group  $H = W/G$  (which is defined in Section A.2), its orbit for  $x \in D_x$  is  $H \cdot x = \{h \cdot x \mid h \in H\}$ . We find that if two elements of  $D_x$ ,  $x_i$  and  $x_j$  have equivalence relation, i.e.,  $\exists h \in H, h \cdot x_i = x_j$ , they are in the same **H-orbit** (brief proof: the orbit of  $x_j$  is  $H \cdot x_j = H \cdot (h \cdot x_i) = Hh \cdot x_i = H \cdot x_i$ , which is actually the orbit of  $x_i$ ). Therefore, for each element in  $D_x$ , we can derive its H-orbit and decide whether it is a new H-orbit or an existed one. After traversing all the elements in  $D_x$ , we can get a partition of  $D_x$  by a bunch of H-orbits. As  $H$  denotes class-agnostic transformations, the equivalent elements in the same H-orbit are in the same class (because  $Hx$  will not change its class according to the definition of  $H$ ). Therefore, the partition of  $D_x$  actually achieves **classification**. Now, we draw the causal graph for classification according to its orbit definition by using the equivalence relation.

**Causal Graph for Classification.** We frame the equivalence relation of H-orbit into causal graph in Figure 1. Note that in this subsection,  $G$  and  $H$  denote variables, while they denote sets in group theory. As the set  $H$  can be derived by sampling variable  $H$  for multiple times, this notation will not lose generality.

$G \rightarrow (X_0, X) \leftarrow H$ .  $G$  is the class-related transformation subgroup of  $W$  and  $H$  is the quotient group (class-agnostic transformation group).  $(X_0, X)$  is an element pair, where elements are from  $D_x$ .  $X$  is transformed from  $X_0$  by  $X = hgX_0$ , where  $g$  and  $h$  are the values of  $G$  and  $H$ . Note that  $X_0$  can be any fixed element in  $D_x$ . Assume  $W$  is transitive on  $D_x$ , for any  $X_0$ , there must exist the corresponding  $g$  and  $h$  to perform the transformation to derive  $X$ .

$(X_0, X) \rightarrow Yes/No \leftarrow H$ . This subgraph describes the judgement for whether  $X$  and  $X_0$  have equivalence relation. For given  $X$ , we need the variable  $H$  provides the value  $h$  and  $H \rightarrow Yes/No$  provides inverse mechanism, to get the following equation:  $h^{-1}X = h^{-1}hgX_0 = gX_0$ . To achieve “Yes” in the judgement, we need further eliminate  $g$  in the RHS.

If  $g = g_i$  is the stabilizer of  $X_0$ , we have  $h^{-1}X = g_iX_0 = X_0$ , which means  $X \sim X_0$  (i.e., they have equivalence relation) under the action  $h$ . Then  $X$  and  $X_0$  are in the same H-orbit with the orbit index  $i$ , which is the index of the given stabilizer  $g_i$  of  $X_0$ . Then, we can define the “class” label  $Y$  by using the judgement, which is an  $n$ -dimension one-hot vector:

$$Y_k = \mathbb{1}_{(h^{-1}X = g_kX_0)}, k = 1, 2, 3, \dots, n, \quad (7)$$

where  $\mathbb{1}$  is the indicator function,  $n$  is the number of stabilizers. Finally, the classification task can be defined as predicting the index  $k$  of H-orbit, which is equivalent to predicting the value of  $Y$ . Now, we have:

**Theorem 2.** According to the causal graph in Figure 1 and classification definition by Eq. (7), **Inverse Probability Weighting** can achieve robustness classification for  $X$ .

**Proof.** Here we use  $X$  to denote the pair  $(X_0, X)$  and use  $Y$  to denote the output of Eq. (7). For robust classification, we need to pursue the causal relationship between  $X$  and  $Y$  (only consider the class features related to  $G$ ). However, as there exists a confounder  $H$  introducing a backdoor path  $(X_0, X) \leftarrow H \rightarrow X_0$ . The traditional probability objective  $P(Y|X)$  will contain the effect of  $H$ , *i.e.*, the context. Therefore, we need to use intervention  $do(X)$  and backdoor adjustment to eliminate the confounder effect from  $H$ . The objective function is written as:

$$\begin{aligned}
P(Y|do(X)) &= \sum_h P(Y|X, h)P(h|X) \\
&= \sum_h P(Y|X, h)P(h) \\
&= \sum_h \frac{P(Y, X, h)}{P(X|h)P(h)} P(h) \\
&= \sum_h P(Y, X, h) \cdot \frac{1}{P(X|h)},
\end{aligned} \tag{8}$$

which is the formula of **Inverse Probability Weighting**, *i.e.*, Eq.3 in the main paper, where  $CE(y_i, \hat{y}_i)$  is the engineering implementation of  $P(Y, X, h)$  and  $\phi_t(x_i)$  is the estimation for  $h$ . Therefore, using ERM-IPW can eliminate the confounder effect of  $H$  in the causal graph and achieve robust classification.

#### A.4 Why does IRMCon realize $\phi_t(x) = x_t$ ?

**Revisit Invariant Risk Minimization (IRM).** We define extractor  $\phi$  as the function mapping from image space to feature space and classifier  $\theta$  as the function mapping from feature space to classification output space. Then, IRM is to optimize:

$$\begin{aligned}
&\min_{\phi, \theta} \sum_e R^e(\theta \cdot \Phi), \\
&\text{subject to } \theta \in \underset{\bar{\theta}}{\operatorname{argmin}} R^e(\bar{\theta} \cdot \Phi) \quad \forall e \in \mathcal{E},
\end{aligned} \tag{9}$$

where  $R^e(\theta \cdot \Phi)$  is the empirical risk in the environment  $e$ ,  $\mathcal{E}$  is the set of environments, and  $\Phi = \phi(x)$  is the representations of input images. The goal of IRM is to simultaneously achieve the optimum of  $\theta$  among all environments. Our IRMCon use the similar implementation just replace  $R^e(\theta \cdot \Phi)$  with contrastive objective  $-\log \frac{\exp(\phi_t(x_i)^T \phi_t(\text{Aug}(x_i)) \cdot \theta)}{\sum_{x'_i \in e} \exp(\phi_t(x_i)^T \phi_t(x'_i) \cdot \theta)}$ . Therefore, our goal is also to achieve the optimum of  $\theta$  simultaneously among different  $e$ . We have the theorem:

**Theorem 3.** *When context  $\mathbf{x}_t$  is shared among environments, if and only if  $\phi_t$  eliminates the environment features, *i.e.*,  $\phi_t(x) = \mathbf{x}_t$ , the IRMCon objective can achieve optimum.*

**Table 1.** Accuracy (%) on context biased datasets. We reproduced all the methods and averaged the results over three independent trials (mean $\pm$ std). Note that, for EnD, we give it ground truth attribute labels (which destroys the settings (no context labels) in context biased datasets) on Colored MNIST and Corrupted Cifar-10, as there are no attribute labels for BAR, we cannot reproduce EnD on BAR.

| Dataset            | Bias Ratio(%) | Methods        |                |                |                |                |                       |
|--------------------|---------------|----------------|----------------|----------------|----------------|----------------|-----------------------|
|                    |               | ERM            | Rebias [3]     | EnD [15]       | LfF [9]        | Feat-Aug [7]   | IRMCon-IPW (Ours)     |
| Colored MNIST      | 99.9          | 20.4 $\pm$ 1.1 | 20.8 $\pm$ 0.6 | 19.8 $\pm$ 1.6 | 56.8 $\pm$ 1.6 | 51.2 $\pm$ 1.8 | <b>66.7</b> $\pm$ 2.3 |
|                    | 99.8          | 26.4 $\pm$ 0.4 | 28.3 $\pm$ 0.9 | 28.1 $\pm$ 0.8 | 68.3 $\pm$ 1.5 | 57.6 $\pm$ 2.6 | <b>75.5</b> $\pm$ 1.5 |
|                    | 99.5          | 42.9 $\pm$ 1.1 | 44.4 $\pm$ 0.5 | 45.1 $\pm$ 1.3 | 77.0 $\pm$ 1.5 | 67.4 $\pm$ 0.3 | <b>81.0</b> $\pm$ 0.9 |
|                    | 99.0          | 59.2 $\pm$ 0.5 | 58.6 $\pm$ 0.4 | 60.2 $\pm$ 0.3 | 82.5 $\pm$ 1.7 | 73.9 $\pm$ 1.9 | <b>85.3</b> $\pm$ 0.3 |
|                    | 98.0          | 72.5 $\pm$ 0.2 | 73.5 $\pm$ 1.0 | 74.7 $\pm$ 1.7 | 84.1 $\pm$ 1.5 | 78.0 $\pm$ 1.5 | <b>88.3</b> $\pm$ 0.2 |
|                    | 95.0          | 85.7 $\pm$ 0.5 | 85.5 $\pm$ 0.5 | 85.4 $\pm$ 0.4 | 86.8 $\pm$ 0.5 | 82.3 $\pm$ 0.1 | <b>92.2</b> $\pm$ 0.5 |
| Corrupted Cifar-10 | 99.5          | 22.7 $\pm$ 0.5 | 22.7 $\pm$ 0.7 | 22.7 $\pm$ 0.6 | 26.1 $\pm$ 0.7 | 29.3 $\pm$ 1.7 | <b>31.0</b> $\pm$ 0.6 |
|                    | 99.0          | 25.8 $\pm$ 0.6 | 24.9 $\pm$ 0.7 | 24.9 $\pm$ 0.7 | 31.8 $\pm$ 0.7 | 35.5 $\pm$ 0.2 | <b>37.1</b> $\pm$ 0.4 |
|                    | 98.0          | 28.7 $\pm$ 0.1 | 29.1 $\pm$ 0.7 | 30.1 $\pm$ 0.7 | 38.9 $\pm$ 1.0 | 41.9 $\pm$ 0.9 | <b>42.5</b> $\pm$ 1.0 |
|                    | 95.0          | 39.9 $\pm$ 1.6 | 38.9 $\pm$ 1.7 | 41.1 $\pm$ 0.8 | 51.3 $\pm$ 0.9 | 52.0 $\pm$ 0.7 | <b>53.8</b> $\pm$ 1.3 |
| BAR                | 99.0          | 52.9 $\pm$ 0.7 | 52.1 $\pm$ 0.5 | -              | 48.1 $\pm$ 2.7 | 41.7 $\pm$ 1.6 | <b>55.3</b> $\pm$ 0.6 |
|                    | 95.0          | 65.2 $\pm$ 1.9 | 65.0 $\pm$ 1.8 | -              | 60.6 $\pm$ 2.6 | 55.8 $\pm$ 2.2 | <b>67.9</b> $\pm$ 0.8 |

**Table 2.** Accuracy (%) of vanilla ERM on BAR compared with ERM (with augmentation) and other methods.

| Dataset | Bias Ratio(%) | Methods        |                |                |                |                       |
|---------|---------------|----------------|----------------|----------------|----------------|-----------------------|
|         |               | ERM (vanilla)  | ERM            | LfF            | Feat-Aug       | IRMCon-IPW            |
| BAR     | 99.0          | 35.2 $\pm$ 2.1 | 52.9 $\pm$ 0.7 | 48.1 $\pm$ 2.7 | 41.7 $\pm$ 1.6 | <b>55.3</b> $\pm$ 0.6 |
|         | 95.0          | 39.7 $\pm$ 1.8 | 65.2 $\pm$ 1.9 | 60.6 $\pm$ 2.6 | 55.8 $\pm$ 2.2 | <b>67.9</b> $\pm$ 0.8 |

**Proof.** If  $\phi_t(x) = \mathbf{x}_t$ , for the contrastive features extracted by  $\phi_t$  in each environment will be same, as context is the only part shared among environments. Therefore, the optimum state of  $\theta^*$  (Note that, although in our implementation  $\theta$  is a constant, it still has optimum state when its gradient is equal to 0) in one environment is still the optimum state in other environments. In contrast, If IRMCon achieves optimum and  $\phi_t$  still encodes the environment features. For each environment  $e = c_i$ , we denote its features by a matrix  $M_\phi^i$ . As the difference between environments is only the class, which can be represented by a transformation matrix  $T_i^j$  (e.g., from  $c_i$  to  $c_j$ ). Then, we can denote the representation matrix for  $c_j$  by a base environment  $c_i$  and a transformation:  $M_\phi^j = T_i^j M_\phi^i$ . As IRMCon achieves optimum, the  $\theta^*$  should be optimal for representations in all environments  $\{M_\phi^k\}_{k=1}^n$ . Therefore the transformations should be the identity matrix, i.e., there is no difference between environments. Otherwise, the contrastive objective cannot achieve optimum simultaneously under varies sets of features by the same  $\theta^*$  (ignoring some trivial cases, where the loss calculation is invariant to the class transformation  $T_i^j$ , excepting  $T_i^j$  is identity). That means the optimum of IRMCon is equivalent to  $\phi_t(x) = \mathbf{x}_t$ .

---

**Algorithm 1: IRMCon-IPW**


---

```

1 Step 1. IRMCon
   Input: Training set  $\{(x_i, y_i)\}_{i=1}^n$ 
   Output: Context feature extractor  $\phi_t$ 
1 Randomly initialize  $\phi_t$ ;
   while not converged do
2   | Sample a mini-batch from training set;
3   | Split it into environments by class label;
4   | Update  $\phi_t$  by IRMCon loss in Eq. 7.;
Step 2. IPW
   Input: Training set  $\{(x_i, y_i)\}_{i=1}^n$ , context feature extractor  $\phi_t$ 
   Output: Context invariance classifier  $f$ 
6 Randomly initialize  $f_b, f, \phi_c$ ;
   while not converged do
7   | Sample a mini-batch from training set;
8   | Use freezed  $\phi_t$  to extract context features  $\mathbf{x}_t$ ;
9   | Estimate  $P(x|\phi_t(x))$  in Eq. 8.
10  | Update  $f_b$  by GCE loss in Eq. 3. with  $\mathbf{x}_t$  as input;
11  | Update  $f, \phi_c$  by ERM-IPW loss in Eq. 3.;

```

---

## B More Experimental Details

### B.1 More Dataset Details

#### Context Biased Datasets.

*Colored MNIST.* We use the dataset generation code from LfF [9], where the images are generated from grayscale digit images in the MNIST dataset, with the size of  $28 \times 28$ . About the detailed generation process, we first choose 10 different RGB values and use this as mean value and use 3-dimensional Gaussian distribution as variance to colorize each grayscale image. We pair digit and color with a correlation ratio selected from  $\{99.9\%, 99.8\%, 99.5\%, 99.0\%, 98.0\%, 95.0\%\}$ . The remaining images are uniformly colorized by the left 9 colors. In the test set, all colors are uniformly distributed over all digits. There are totally 60,000 training images and 10,000 test images in each setting.

*Corrupted CIFAR-10.* We also use the dataset generation code from LfF [9], where the images are generated from Cifar-10 Dataset, with the size of  $32 \times 32$ . Here, we set the attribute as 10 different corruptions  $\{\text{Saturate, Elastic, Impulse, Brightness, Contrast, Gaussian, Defocus Blur, Pixelate, Gaussian Blur, Frost}\}$ , and other generation protocols are the same as the Colored MNIST. We totally set four correlation ratios  $\{99.5\%, 99.0\%, 98.0\%, 95.0\%\}$ , and in each setting, there are totally 50,000 training images and 10,000 test images.

*Biased action recognition dataset (BAR).* This dataset is proposed by LfF [9], which contains 6 kinds of action-place bias:  $\{(\text{Climbing, RockWall}), (\text{Diving, Underwater}), (\text{Fishing, WaterSurface}), (\text{Racing, APavedTrack}), (\text{Throwing, PlayingField}), (\text{Vaulting, Sky})\}$ . There are totally 1,941 biased images and 654 unbi-

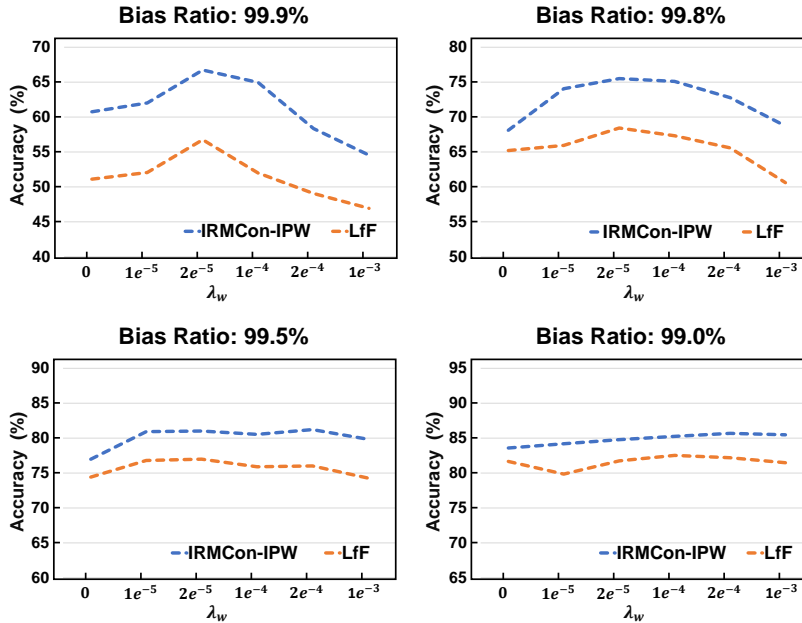

**Fig. 3.** The test accuracy (%) of LfF [9] and our IRMCon-IPW with different values of  $\lambda_w$  trained on 4 biased Colored MNIST datasets. The results show that we always outperform LfF under any setting.

ased images in the dataset. We set the ratio of biased images in the training set ranging in  $\{99.0\%, 95.0\%\}$ , that means we select 17 unbiased images to create 99.0% biased settings, where there are 1.958 training images and 637 test images; and we select 94 unbiased images to create 95.0% biased settings, where there are 2,035 training images and 560 test images.

**Domain Gap Datasets.** In the domain generalization task, we follow DOMAINBED [4] to preprocess the dataset and the input image size is set to  $224 \times 224$  for all settings. All dataset details are the same as the DOMAINBED [4] code base.

## B.2 More Implementation Details

In this section, we provide more implementation details. We set batch size as 256, 256 and 64 for *Colored MNIST*, *Corrupted Cifar-10* and *BAR*, respectively. We totally train 50, 50 and 250 epochs for *Colored MNIST*, *Corrupted Cifar-10* and *BAR*, respectively. For *PACS*, we apply Adam optimizer with 0.001 learning rate for 100 epochs training from scratch for all the methods. To save space, if the hyperparameters are different in each setting under a dataset, we narrate them by the following orders: Colored MNIST is  $\{99.9\%, 99.8\%, 99.5\%, 99.0\%, 98.0\%, 95.0\%\}$ ; Corrupted Cifar-10 is  $\{99.5\%, 99.0\%, 98.0\%, 95.0\%\}$ ; BAR is  $\{99.0\%, 95.0\%\}$ ; PACS is  $\{\text{“art painting”}, \text{“cartoon”}, \text{“photo”}, \text{“sketch”}\}$ .

**Table 3.** Accuracy (%) on domain gap datasets with pretrained ResNet-18. We reproduced the methods by the DOMAINBED [4] code base and results are averaged over three independent trials (mean $\pm$ std). “-” denotes the implementation issue in the training.

|                        | Methods       | PACS           |                |                |                |      |
|------------------------|---------------|----------------|----------------|----------------|----------------|------|
|                        |               | Art.           | Cartoon        | Photo          | Sketch         | Avg. |
| w/ domain supervision  | IRM[2]        | 80.0 $\pm$ 0.7 | 76.9 $\pm$ 0.3 | 95.5 $\pm$ 0.4 | 72.6 $\pm$ 0.9 | 81.2 |
|                        | DRO [12]      | 81.8 $\pm$ 0.4 | 75.9 $\pm$ 0.5 | 95.6 $\pm$ 0.4 | 75.9 $\pm$ 1.1 | 82.3 |
|                        | InterMix [17] | 81.7 $\pm$ 0.5 | 74.7 $\pm$ 0.5 | 95.3 $\pm$ 0.1 | 70.7 $\pm$ 0.4 | 80.6 |
|                        | MLDG [8]      | 82.0 $\pm$ 0.6 | 76.5 $\pm$ 0.4 | 96.1 $\pm$ 0.4 | 76.1 $\pm$ 0.8 | 82.6 |
|                        | DANN [1]      | 53.5 $\pm$ 3.1 | 63.3 $\pm$ 2.9 | 90.0 $\pm$ 0.2 | 60.4 $\pm$ 1.5 | 66.8 |
|                        | V-REx [6]     | 81.4 $\pm$ 0.6 | 77.2 $\pm$ 0.6 | 95.1 $\pm$ 0.1 | 77.6 $\pm$ 0.7 | 82.8 |
|                        | Fish [14]     | 81.3 $\pm$ 0.1 | 76.9 $\pm$ 0.5 | 96.0 $\pm$ 0.1 | 74.8 $\pm$ 0.1 | 82.2 |
|                        | TRM [16]      | 83.6 $\pm$ 1.7 | 77.9 $\pm$ 0.5 | -              | 75.7 $\pm$ 1.3 | -    |
| w/o domain supervision | ERM           | 80.3 $\pm$ 0.3 | 76.4 $\pm$ 0.4 | 95.4 $\pm$ 0.4 | 76.5 $\pm$ 0.4 | 82.1 |
|                        | SD [11]       | 83.9 $\pm$ 0.2 | 78.5 $\pm$ 0.3 | 95.9 $\pm$ 0.1 | 75.3 $\pm$ 0.4 | 83.4 |
|                        | RSC [5]       | 75.2 $\pm$ 0.4 | 74.7 $\pm$ 0.7 | 93.0 $\pm$ 0.4 | 71.4 $\pm$ 1.4 | 78.6 |
|                        | LfF [9]       | 80.4 $\pm$ 0.4 | 76.8 $\pm$ 1.3 | 95.3 $\pm$ 0.3 | 72.5 $\pm$ 0.9 | 81.2 |
|                        | IRMCon-IPW    | 81.1 $\pm$ 0.4 | 77.3 $\pm$ 1.3 | 95.4 $\pm$ 0.3 | 76.6 $\pm$ 1.3 | 82.6 |

For our IRMCon, we apply the same backbone as LfF bias model, with a contrastive head, where the contrastive head dimension is 12 for Colored MNIST and 64 for others. Under the weighted sample strategy, we train IRMCon by 0.4k, 8k, 1.6k iterations for Colored MNIST, Corrupted Cifar-10 and BAR respectively, the optimization is by Adam with learning rate as 0.008, 0.002, 0.002, 8e-4 for Colored MNIST, Corrupted Cifar-10, BAR and domain gap datasets. For  $\lambda$ , we set it as 1.0 for context biased datasets and 0.1 for domain gap datasets. Note that  $f_b$  in Eq. 4 for LfF in the main paper is the classification head of the backbone;  $f_b$  in Eq. 8 for ours is a 2 layer MLP, where the input dimension is our contrastive feature (context) dimension and middle dimension is  $8 \times$  input dimension for Colored MNIST and  $2 \times$  input dimension for others.

We provide the ablation study for  $\lambda$  (in Eq. 7 in the main paper) on Colored MNIST in Table 4. The results show that the regularization term helps us realize better context disentanglement and finally improve the OOD generalization performance, but higher regularization weights sometimes influence the optimization (See the performance on 99.9% biased Colored MNIST, when we set  $\lambda = 5.0$ .) Besides, in the implementation for Eq. 4 in the main paper, we find a 0-value problem of the weight estimation formula. For example, when training the 99.5% biased Colored MNIST, We find 33,400 0-value weights estimated by LfF bias model, over 60,000 at epoch 5. This means unbiased model will lose many possible valuable samples in the whole training process, leading to the inferior perfor-

**Table 4.** Accuracy (%) of IRMCon-IPW on Colored MNIST dataset with different values of  $\lambda$ . In the main paper, we report the results when  $\lambda = 1.0$ .

| Bias(%) | $\lambda$      |                       |                       |                |
|---------|----------------|-----------------------|-----------------------|----------------|
|         | 0.0            | 1.0                   | 2.0                   | 5.0            |
| 99.9    | 60.1 $\pm$ 1.3 | <b>66.7</b> $\pm$ 2.3 | 64.7 $\pm$ 0.7        | 58.8 $\pm$ 6.4 |
| 99.8    | 73.8 $\pm$ 1.4 | <b>75.5</b> $\pm$ 1.5 | 73.4 $\pm$ 0.8        | 72.6 $\pm$ 1.2 |
| 99.5    | 79.3 $\pm$ 2.6 | 81.0 $\pm$ 0.9        | <b>81.1</b> $\pm$ 0.9 | 80.3 $\pm$ 1.0 |
| 99.0    | 84.8 $\pm$ 0.6 | 85.3 $\pm$ 0.3        | <b>86.2</b> $\pm$ 0.7 | 85.7 $\pm$ 0.1 |
| 98.0    | 87.9 $\pm$ 0.2 | 88.3 $\pm$ 0.2        | <b>88.5</b> $\pm$ 0.2 | 88.2 $\pm$ 0.6 |
| 95.0    | 91.8 $\pm$ 0.1 | <b>92.2</b> $\pm$ 0.5 | 91.9 $\pm$ 0.1        | 91.5 $\pm$ 0.2 |

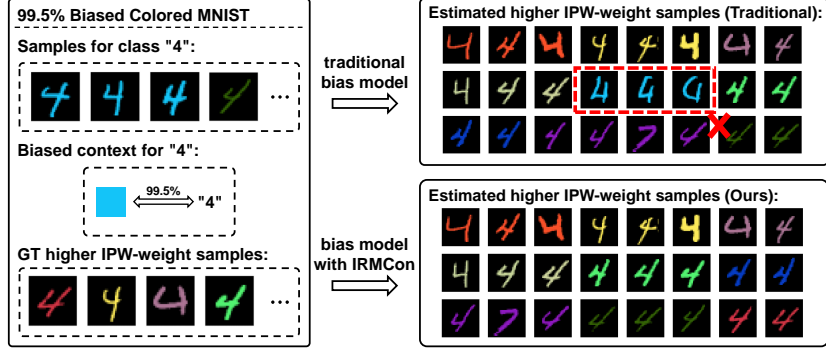

**Fig. 4.** Visualization for the samples with higher weights generated by traditional method (LfF [9], *Top*) and ours (*Bottom*). As “blue” context is the dominating context for class “4”, model should assign higher weights for other color samples and lower weights for “blue” samples. The traditional method wrongly assigns higher weights for some “blue” samples because of the failure classification, while ours can derive the right context weights because we eliminate the class information by IRMCon and only generate weights by the context rarity.

mance. As a result, we add a  $\lambda_w$  on Eq. 8 to improve the weight estimation formula to ignore 0-value weight problem. To justify our improvement is not only from the improvement of weight estimation formula, we compare our method and LfF under different  $\lambda_w$  under several settings on Colored MNIST in Fig. 3. We find that although LfF can also be improved by our refined weight estimation formula, our IRMCon-IPW always outperform LfF under any settings with different  $\lambda_w$ , which means the key improvement of our method is the better context estimation, *i.e.*,  $\lambda_w$  only play a role as assist.

### B.3 How does our IRMCon-IPW superior to the traditional context estimation methods

*The failure of traditional methods.* As the traditional methods, such as LfF [9], use class classification results to estimate context, its context estimation is destined to be mixed with class. In another viewpoint, the reweighting implementation of LfF can be seen as finding hard samples and assigning higher weights to them. For example, the samples with rare context are hard samples (in 99.5% Colored MNIST, there is only 0.5% samples with other colors, called **context rare** samples). However, there is another case that the samples with bad class features are also hard samples (as shown in Fig. 4 red box, called **class noisy** samples). It is right to assign higher weights for the **context rare** samples, but not for the **class noisy** samples, which will degenerate the reweighting performance. This is also the reason for Fig. 6. (Bottom) in the main paper. If there is no context bias, *i.e.*, no **context rare** samples, no one should be

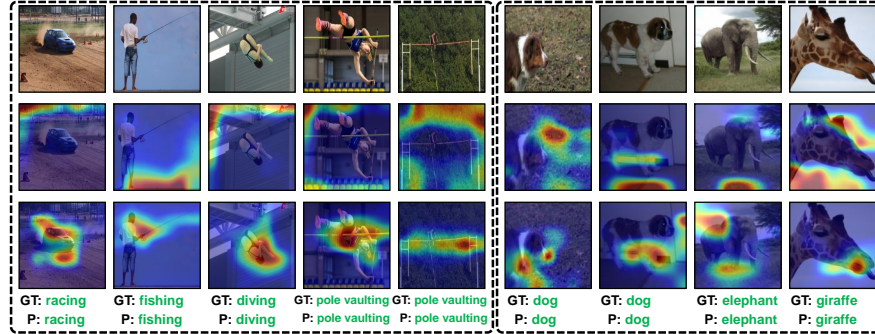

**Fig. 5.** GradCAM [13] visualizations of IRMCon-IPW successful cases. Top: input test images, Middle: context visualization by bias classifier of IRMCon, Bottom: class visualization of model trained by IRMCon-IPW. Left five samples are selected from BAR test set, model is trained on the 99% biased training set; right four are selected from photo domain of PACS, model is trained on the left three domains.

assigned with higher weights. For the traditional reweighting methods, the **class noisy** samples still exist, and the model will assign higher weights to them. The result is model wrongly learns some **class noisy** samples with higher weights and degenerates the performance, which is even worse than the ERM baseline.

*The superiority of our IRMCon-IPW.* Thanks to our IRMCon, we can realize accurate context estimation, *i.e.*, disentangling context by eliminating class. Therefore, our context bias estimation classifier is from context to class label, the correlation between context and class is the only way for optimization. For example, in the 99.5% biased Colored MNIST, our classifier can use context correlation to achieve accurate 99.5% accuracy (Illustrated in Fig. 7 (Top) in the main paper). As our classifier is only relying on context correlation to classify, in the test set, the classifier will only achieve 10% accuracy (randomly guess) because there is no context correlation in the test set. Due to the accurate context estimation, our hard examples are only **context rare** samples, which is illustrated in Fig. 4 right bottom. Therefore, we can perform better reweighting process by only assigning higher weights to the context rare samples. In the balanced training setting in Fig. 6. in the main paper, as there is no correlation between our inputs (context) and labels (class), the bias model will learn nothing. In the practice, the loss of bias, *i.e.*,  $CE(y, \hat{y} = f_b(\mathbf{x}_t))$  in Eq. 8 in the main paper, will not decrease, which is much larger than  $CE(y, \hat{y} = f(\phi_c(x)))$ . Therefore, the weight for every sample is nearly 1 and our IRMCon-IPW can perform similarly compared to the ERM baseline. This is the reason for Fig. 6 (Bottom), that our IRMCon-IPW achieves comparable performance to ERM in the context balanced setting.

## C More Quantitative Results

### C.1 Results on Context Biased Dataset

In Table 1, we provide the reproduced results of Feat-Aug [7] and End [15], compared with ERM and IRMCon-IPW (ours).

### C.2 Results for vanilla ERM on BAR

In Table 2, we provide the results of vanilla ERM on BAR. The results show that, without strong augmentation, especially the RandCrop transformation, the performance of ERM drops severely.

### C.3 Results on Domain Gap Dataset

In Table 3, we provide the results on Domain Gap Dataset with pretrained ResNet-18. All methods are trained for 30 epochs with Adam optimizer, the learning rate is  $5e-5$ . The result shows that, our IRMCon-IPW can still improve ERM and be comparable to the SOTA method. Note that we provide the performance of pretrained setting just for reference, as we mentioned that pretraining setting meets the data leakage problem.

## D More Qualitative Results

In Figure 5, we show some successful examples for IRMCon-IPW, where IRMCon correctly estimates the context and IRMCon-IPW successfully predicts the right classification result.

## References

1. Ajakan, H., Germain, P., Larochelle, H., Laviolette, F., Marchand, M.: Domain-adversarial neural networks. In: NIPS (2014)
2. Arjovsky, M., Bottou, L., Gulrajani, I., Lopez-Paz, D.: Invariant risk minimization. arXiv preprint arXiv:1907.02893 (2019)
3. Bahng, H., Chun, S., Yun, S., Choo, J., Oh, S.J.: Learning de-biased representations with biased representations. In: ICML (2020)
4. Gulrajani, I., Lopez-Paz, D.: In search of lost domain generalization. In: ICLR (2021)
5. Huang, Z., Wang, H., Xing, E.P., Huang, D.: Self-challenging improves cross-domain generalization. In: ECCV (2020)
6. Krueger, D., Caballero, E., Jacobsen, J.H., Zhang, A., Binas, J., Zhang, D., Le Priol, R., Courville, A.: Out-of-distribution generalization via risk extrapolation (rex). In: International Conference on Machine Learning (2021)
7. Lee, J., Kim, E., Lee, J., Lee, J., Choo, J.: Learning debiased representation via disentangled feature augmentation. In: NIPS (2021)

8. Li, D., Yang, Y., Song, Y.Z., Hospedales, T.M.: Learning to generalize: Meta-learning for domain generalization. In: Thirty-Second AAAI Conference on Artificial Intelligence (2018)
9. Nam, J., Cha, H., Ahn, S., Lee, J., Shin, J.: Learning from failure: Training debiased classifier from biased classifier. In: NIPS (2020)
10. Pearl, J., Glymour, M., Jewell, N.P.: Causal inference in statistics: A primer. John Wiley & Sons (2016)
11. Pezeshki, M., Kaba, S.O., Bengio, Y., Courville, A., Precup, D., Lajoie, G.: Gradient starvation: A learning proclivity in neural networks. In: NIPS (2021)
12. Sagawa, S., Koh, P.W., Hashimoto, T.B., Liang, P.: Distributionally robust neural networks for group shifts: On the importance of regularization for worst-case generalization. In: ICLR (2020)
13. Selvaraju, R.R., Cogswell, M., Das, A., Vedantam, R., Parikh, D., Batra, D.: Grad-cam: Visual explanations from deep networks via gradient-based localization. In: ICCV (2017)
14. Shi, Y., Seely, J., Torr, P.H., Siddharth, N., Hannun, A., Usunier, N., Synnaeve, G.: Gradient matching for domain generalization. arXiv preprint arXiv:2104.09937 (2021)
15. Tartaglione, E., Barbano, C.A., Grangetto, M.: End: Entangling and disentangling deep representations for bias correction. In: CVPR (2021)
16. Xu, Y., Jaakkola, T.: Learning representations that support robust transfer of predictors. arXiv preprint arXiv:2110.09940 (2021)
17. Yan, S., Song, H., Li, N., Zou, L., Ren, L.: Improve unsupervised domain adaptation with mixup training. arXiv preprint arXiv:2001.00677 (2020)
